# Supplementary material for: Effect of uniaxial stress on helimagnetic phases in the square-lattice itinerant magnet EuAl$_{4}$
Source: arXiv:2511.07079 source file (2026-03-09)
Supplement: Supplementary file 1 [file EuAl4_US_supple.tex]

\documentclass[reprint,superscriptaddress,aps]{revtex4-1}
\usepackage{amsmath}
\usepackage{amssymb}
\usepackage{bm}
\usepackage{braket}
\usepackage{color}
\usepackage[varg]{txfonts}
\usepackage{here}
\usepackage{varwidth}
\usepackage{dcolumn}
\usepackage[breaklinks,colorlinks=true,linkcolor=blue,urlcolor=cyan,citecolor=blue]{hyperref}
\setcounter{equation}{0}

\setcounter{figure}{0}

\setcounter{table}{0}

\usepackage{graphicx}

\begin{document}

\title{Supplemental Material for\\``Effect of uniaxial stress on helimagnetic phases in the square-lattice itinerant magnet EuAl$_{4}$"}

\author{Masaki Gen}
\email{gen@issp.u-tokyo.ac.jp}
\affiliation{Institute for Solid State Physics, University of Tokyo, Kashiwa 277-8581, Japan}
\affiliation{RIKEN Center for Emergent Matter Science (CEMS), Wako 351-0198, Japan}

\author{Takuya Nomoto}
\affiliation{Department of Physics, Tokyo Metropolitan University, Hachioji, Tokyo 192-0397, Japan}

\author{Hiraku~Saito}
\affiliation{Institute for Solid State Physics, University of Tokyo, Kashiwa 277-8581, Japan}

\author{Taro~Nakajima}
\affiliation{Institute for Solid State Physics, University of Tokyo, Kashiwa 277-8581, Japan}
\affiliation{RIKEN Center for Emergent Matter Science (CEMS), Wako 351-0198, Japan}
\affiliation{Institute of Materials Structure Science, High Energy Accelerator Research Organization, Tsukuba 305-0801, Japan}

\author{Yusuke~Tokunaga}
\affiliation{Department of Advanced Materials Science, The University of Tokyo, Kashiwa 277-8561, Japan}

\author{Rina~Takagi}
\affiliation{Institute for Solid State Physics, University of Tokyo, Kashiwa 277-8581, Japan}

\author{Shinichiro~Seki}
\affiliation{Research Center for Advanced Science and Technology, University of Tokyo, Tokyo 113-8656, Japan}
\affiliation{Department of Applied Physics, The University of Tokyo, Tokyo 113-8656, Japan}

\author{Taka-hisa~Arima}
\affiliation{RIKEN Center for Emergent Matter Science (CEMS), Wako 351-0198, Japan}
\affiliation{Department of Advanced Materials Science, The University of Tokyo, Kashiwa 277-8561, Japan}

\maketitle
%%%%%%%%%%%%%%%%%%%%%%%%%%%%%%%%%%%%%%%%%%%%%%%%%%%%%%%%

\onecolumngrid

\vspace{+0.5cm}
\subsection*{\label{Sec1} \large Note 1. Experiments under compressive uniaxial stress}

In this study, we used home-built probes equipped with a clamp-type uniaxal-stress cell \cite{2011_Nak, 2015_Nakajima, 2015_Nii, 2018_Nak, 2023_Sai} to apply compressive stress $\sigma_{[010]}$ along the [010] direction, enabling in situ, isothermal control of the applied stress at low temperatures.
We prepared two pieces of rectangular-parallelepiped-shaped single crystals, \#A and \#B, with dimensions $2.0 \times 1.5 \times 0.5$~mm$^{3}$ and $1.8 \times 1.3 \times 0.9$~mm$^{3}$, respectively.
Crystal \#A was used for resistivity measurements and neutron scattering scattering experiments, while crystal \#B was used for magnetization measurements.

The resistivity was measured using the standard four-probe method with the current $I \parallel [100]$ under vertical stress $\sigma_{[010]}$ in a commercial cryostat equipped with a superconducting magnet (PPMS, Quantum Design).
A photograph of the sample setup is shown in Fig.~\ref{FigS1}(a).
Measurements were performed between 8 and 20 K at each applied stress, with a temperature sweep rate of 0.1 K/min on warming.

The magnetization was measured under horizontal stress $\sigma_{[010]}$ with $H \parallel [001]$ using a commercial SQUID magnetometer (MPMS-XL, Quantum Design).
A photograph of the sample setup is shown in Fig.~\ref{FigS1}(b).
Data were acquired in DC mode at each set temperature and field.

Neutron scattering experiments were performed under vertical stress $\sigma_{[010]}$ with a triple-axis spectrometer (PONTA, 5G) at JRR-3, Japan Atomic Energy Agency \cite{2024_Nak}.
The spectrometer was operated in the two-axis mode with a horizontal collimation of 120'-80'-80'-120'.
An incident neutron beam with a wavelength of 1.64~$\AA$ was obtained by a pyrolytic graphite (002) monochromator.

\begin{figure}[b]
\centering
\vspace{+0.5cm}
\includegraphics[width=0.95\linewidth]{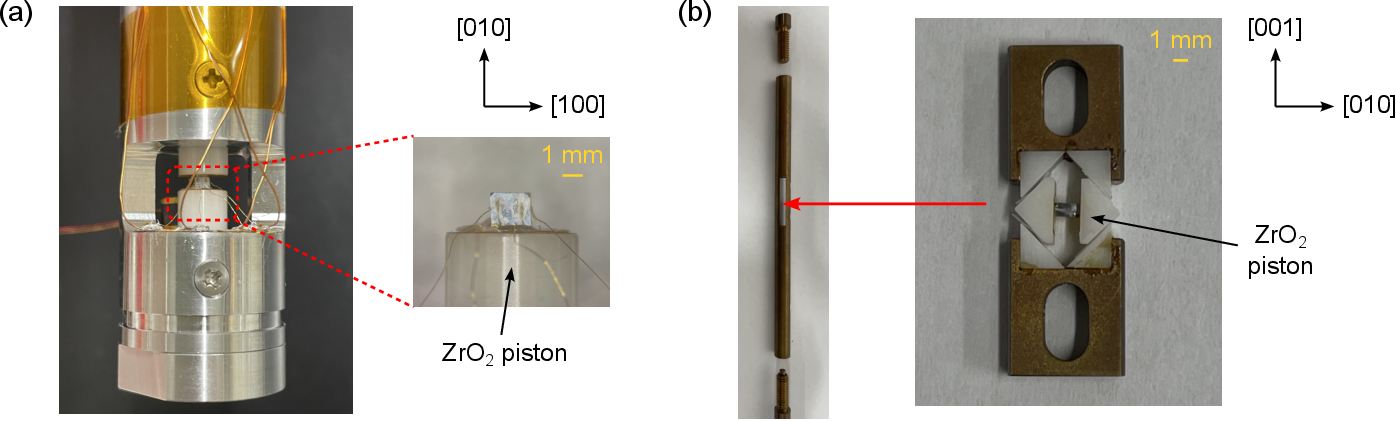}
\caption{Photographs of the sample setup for (a) resistivity and (b) magnetization measurements under uniaxial stress $\sigma_{[010]}$.}
\label{FigS1}
\end{figure}

\newpage
\subsection*{\label{Sec2} \large Note 2. Details of first-principles calculations}

Density functional theory calculations were performed for EuAl$_{4}$ using the projector augmented-wave method as
implemented in the Vienna Ab initio Simulation Package \cite{1996_Kre}.
The exchange-correlation effects were treated within the generalized gradient approximation formulated by Perdew, Burke, and Ernzerhof \cite{1996_Per}.
All calculations were carried out with a plane-wave energy cutoff of 500~eV and a $12 \times 12 \times 12$ Monkhorst-Pack $k$-point mesh.
For europium, an open-core pseudopotential corresponding to the Eu$^{2+}$ ion was employed.
Structural optimization was first conducted at zero pressure, followed by calculations under various lattice distortions to determine the elastic constants $C_{11}$, $C_{12}$, $C_{13}$, and $C_{33}$.
Subsequently, uniaxial-stress calculations were performed using the distorted lattice parameters estimated from the elastic constants [Fig.~4(c)], and the corresponding electronic structures were obtained.
The Fermi surfaces (FSs) shown in Figs.~4(a), 4(b) and Figs.~\ref{FigS2}(a), \ref{FigS2}(b) were obtained using Wannier interpolation with the Wannier90 code \cite{2014_Mos} and a dense $k$-point mesh.

Figures~\ref{FigS2} shows the calculated FS for band \#2 (see the main text for details).
As shown in Fig.~\ref{FigS2}(b), two star-shaped FSs are formed around the $\Gamma$ point.
The corresponding nesting vectors are $q_{x} = 0.36$ and $q_{x}' = 0.07$, neither of which is consistent with the magnetic modulation vector ${\mathbf Q} = (0.19, 0, 0)$ in phase~I.

\begin{figure}[h]
\centering
\vspace{+0.5cm}
\includegraphics[width=0.6\linewidth]{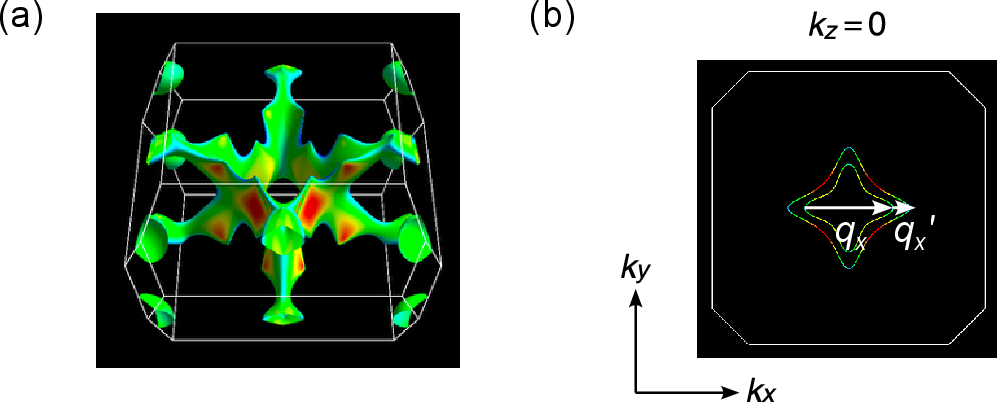}
\caption{Calculated Fermi surfaces (FSs) for band \#2 of EuAl$_{4}$. Panel (b) shows the FSs near the $\Gamma$ point within the $k_{x}$--$k_{y}$ plane.}
\label{FigS2}
\end{figure}

\vspace{+2.0cm}

\end{document}
